# Supplementary material for: Relaxation dynamics induced in glasses by the absorption of hard X-ray photons
Source: arXiv:1902.11027 ancillary file (2019-02-28)
Supplement: Supplementary file 1 [file supp_bis.pdf]

# Supplementary Material for
# "Relaxation dynamics induced in glasses by the absorption of hard X-ray photons"

G. Pintori[1], G. Baldi[1], B. Ruta[2,3] and G. Monaco[1]
[1] *Dipartimento di Fisica, Trento University, Povo, Trento I-38123, Italy*
[2] *ESRF–The European Synchrotron, CS40220, 38043 Grenoble, France*
[3] *Institut Lumière Matière, UMR5306 Université Lyon 1-CNRS, Université de Lyon, 69622 Villeurbanne Cedex, France*
(Dated: October 13, 2017)

## SAMPLE PREPARATION

The $B_2O_3$ glass used in this study was prepared starting from 99%–purity $B_2O_3$ powder (Sigma-Aldrich), which was heated at 423 K and there kept for 16 h to reduce the water content. Water has in fact a large effect on the properties of the $B_2O_3$ glass [1]. For example, the presence of 1 wt% water in this glass decreases the structural relaxation time by an order of magnitude at the glass transition temperature $T_g$ [2]. This makes it very difficult to quantitatively compare the results of different studies due to the uncertainties in the water content in the samples used. The dehydrated powder was melted in air in an alumina crucible and a clear bubble free melt was obtained after 4 h at 1230 K. It was quickly cooled to room-temperature to produce a glass, with a cooling rate of the order of 10 $K/s$. On cooling down, the melt was pressed between two metallic plates and then polished down to achieve a thickness $L = 180 \pm 20$ $\mu m$. This thickness was chosen to optimize the scattered intensity at 8.1 keV while keeping a reasonably good contrast in the wide angle geometry.

## SETUP FOR THE X-RAY PHOTON CORRELATION EXPERIMENT

The XPCS measurements were performed at beamline ID10 at the ESRF in Grenoble (F). The 8.1 keV X-ray beam, produced by an undulator source, was monochromatized using a Si(111) channel-cut (energy bandwidth $\Delta E/E \approx 1.4 \times 10^{-4}$) and then focused by a Be compound refractive lens at the sample position. Hard X-rays originating from higher order monochromator reflections were suppressed by a white beam double mirror placed before the main monochromator. The spatially coherent part of the beam was selected by rollerblade slits opened to 10(H)×8(V) $\mu m^2$, placed $\sim$ 0.18 m upstream of the sample. This configuration leads to a beam with a longitudinal coherence length of $\sim$1.1 $\mu m$ and a transverse coherence length of $\sim$4 $\mu m$ (H)×10 $\mu m$ (V). The speckle patterns were collected by two IkonM charge–coupled devices (CCD) from Andor Technology (1024×1024 pixels, 13×13 $\mu m^2$ pixel size) installed perpendicularly to the horizontal scattering plane, $\sim$67 cm downstream of the sample, and symmetrically arranged with respect to the incoming beam. The CCDs were both centered at a scattering angle corresponding to the maximum of the structure factor $Q_{max}$=1.5 $Å^{-1}$. All pixels of the CCDs were associated to the same wave vector $Q_{max}$ with a resolution of $\Delta Q = 0.04$ $Å^{-1}$.

A resistively heated furnace in vacuum was used for the experiment. The XPCS measurements were carried out in transmission geometry. The temperature was measured by a thermocouple placed close to the sample and was monitored during the whole experiment. The temperature stability was ±0.05 K.

## X-RAYS EFFECT ON THE STRUCTURE

We periodically measured the Q-dependence of the scattered intensity I(Q) to check that radiation damage was not altering the sample. In Figure 1 we report, as an example, the I(Q) data measured on the same spot at the beginning and at the end of an XPCS scan, corresponding in this case to an accumulated dose of 2.2 GGy. As it can be seen, the scattered intensity is stable with 2% accuracy. We can therefore conclude that radiation damage is negligibly altering the structure up to these doses.

[1] M. A. Ramos, J. A. Moreno, S. Vieira, C. Prieto, J. F. Fernández, J. Non-Cryst. Solids **221**, 170 (1997).
[2] J. A. Bucaro, H. D. Dardy, J. Appl. Phys. **45**, 2121 (1974).

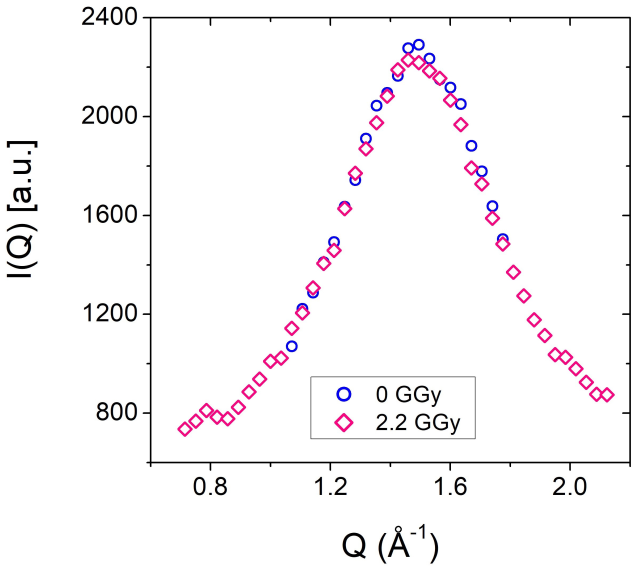


FIG. 1: Total scattered intensity profile measured in $B_2O_3$ on a fresh spot (circles) and after a dose of $\sim$ 2.2 GGy (lozenges). The data are normalized by the incoming beam intensity after background subtraction.
